# Supplementary material for: Effect of stretching-induced changes in hydrodynamic screening on coil-stretch hysteresis of unentangled polymer solutions
Source: arXiv:1609.01796 source file (2016-09-07)
Supplement: Supplementary file 1 [file suppmatl-v1.pdf]

# Supplementary Information for "Effect of stretching-induced changes in hydrodynamic screening on coil–stretch hysteresis of unentangled polymer solutions"

Ranganathan Prabhakar,[1] Chandi Sasmal,[2] Duc At Nguyen,[2] Tam Sridhar,[2] and J. Ravi Prakash[2]

[1]*Department of Mechanical & Aerospace Engineering, Monash University, Clayton, VIC 3800, AUSTRALIA*

*email: prabhakar.ranganathan@monash.edu*

[2]*Department of Chemical Engineering, Monash University, Clayton, VIC 3800, AUSTRALIA*

(Dated: September 6, 2016)

## Abstract

PACS numbers: 83.80.Rs, 83.50.Jf, 83.10.Gr, 47.50.Cd, 47.57.Ng

## STANDARD DEFINITIONS

The average diameter of a flexible polymer coil at equilibrium in a theta solvent is $R_0$, while Its contour length is $L$. The number of Kuhn segments, $N_{\mathrm{K}} = L^2/R_0^2$, and the length of a single Kuhn segment is $b_{\mathrm{K}} = R_0^2/L$. The hydrodynamic radius of a single Kuhn segment is $a_{\mathrm{K}}$ so that its friction coefficient is $6\pi\,\eta_{\mathrm{s}}\,a_{\mathrm{K}}$, where $\eta_{\mathrm{s}}$ is the solvent viscosity. The hydrodynamic interaction parameter corresponding to $a_{\mathrm{K}}$ is defined as

$$h_{\mathrm{K}}^* = \frac{a_{\mathrm{K}}}{\sqrt{\pi}\,b_{\mathrm{K}}}\,. \tag{1}$$

The average friction coefficient of equilibrium coils at infinite dilution is referred to as the Zimm friction coefficient and is denoted as $\zeta_{\mathrm{Z}}$. In the absence of intramolecular hydrodynamic interaction (for instance, when it is completely screened by the presence of neighbouring chains), chains are freely draining with a Rouse friction $\zeta_{\mathrm{R}} = 6\pi\,\eta_{\mathrm{s}}\,a_{\mathrm{K}}\,N_{\mathrm{K}} = 6\pi^{3/2}\,h_{\mathrm{K}}^*\,\eta_{\mathrm{s}}\,L$. Equilibrium coils begin interpenetrate at a chain number density $c^*$, referred to as the critical overlap concentration. From a scaling perspective, $c^* \sim R_0^{-3}$.

## EXPERIMENTAL POLYMER SOLUTIONS

Experiments were performed with high-molecular-weight polystyrene of molecular weight $M_w$ = 978 kDa, which corresponds to $N_{\mathrm{K}}$ = 1318 (based on an estimate of 742 Da per Kuhn segment from bond angle and stiffness [1]). Two different mixtures of dioctylphthalate and oligomeric styrene (Piccolastic A5 from Eastman Chemical) were chosen to obtain solvents of different shear viscosities. The preparation methods are described by Gupta et al. [2]. The composition and shear properties of these solutions are shown in the table below. The modulus $c\,k_{\mathrm{B}}T = c_{\mathrm{m}}RT/M_w$, where $c$ is the chain number density, $c_{\mathrm{m}}$ is the mass concentration, $R$ = 8.314 J/ (mol K) is the universal gas constant, and $T$ = 295 K is the room temperature. The critical overlap concentration for these solutions is estimated from the zero-shear-rate intrinsic viscosity $[\eta]_0$ using Graessley's [1980] relation:

$$c_{\mathrm{m}}^* = \frac{0.77}{[\eta]_0}\,. \tag{2}$$

The relaxation time $\lambda_0$ was estimated from the low-frequency ($\omega$) asymptote of the elastic modulus $G'$ obtained by small-amplitude oscillatory shear experiments as

$$\lambda_0 = \lim_{\omega\to 0} \frac{G'}{\eta_{\mathrm{p},0}\,\omega^2}\,,$$

where $\eta_{\mathrm{p},0} = \eta_0 - \eta_{\mathrm{s}}$ is the polymer contribution the zero-shear rate viscosity $\eta_0$, and $\eta_{\mathrm{s}}$ is the solvent viscosity.

TABLE I. Parameters for polystyrene solutions

| $c_{\mathrm{m}}$ | $c\,k_{\mathrm{B}}T$ | $c/c^*$ | $\eta_0$ | $\eta_{\mathrm{s}}$ | $\lambda_0$ |
|---|---|---|---|---|---|
| g/L | Pa | - | Pa s | Pa s | s |
| 0.52 | 1.31 | 0.05 | 28.4 | 26.2 | 0.60 |
| 3.13 | 7.85 | 0.3 | 41.6 | 26.2 | 0.61 |
| 4.07 | 10.2 | 0.4 | 46.4 | 26.2 | 0.57 |
| 5.21 | 13.1 | 0.5 | 51.1 | 26.2 | 0.60 |
| 12.4 | 31.1 | 1.3 | 103.7 | 26.2 | 0.98 |
| 45.6 | 114.3 | 4.7 | 75.7 | 1 | 0.32 |

## MULTI-CHAIN BROWNIAN DYNAMICS SIMULATIONS

A polymer solution at finite concentration is modelled as an ensemble of polymer chains represented by a linear bead spring chain model, immersed in an incompressible Newtonian solvent. Each polymer molecule is coarse-grained into a linear chain of $N_b$ beads connected by $N_s (= N_b - 1)$ massless Finitely Extensible Nonlinear Elastic (FENE) springs. The simulation box is a cube of edge length $L$ in which a total of $N_c$ chains are enclosed, resulting in a total of $N = N_b \times N_c$ beads per box at a bulk concentration of $c = N/V$, where $V = L^3$ is the volume of the simulation cell. The numerical method used to integrate the Ito stochastic differential equations governing the position vectors of the beads is described in Refs. [4] and [5]. An optimized Ewald-sum algorithm was used to evaluate the mobility matrix and its square-root decomposition in the multiplicative noise term. This algorithm was combined with the Kraynik-Reinhelt algorithm for periodic boundary conditions in planar extensional flows, as presented by Jain et al. [5]. The parameter governing the strength of the inter-bead hydrodynamic interaction is $h^*$ which is effectively the dimensionless hydrodynamic radius of each bead.

For a planar extensional flow where the principal stretching direction is along the $x$-axis,

the transpose of the velocity gradient tensor is

$$\boldsymbol{\kappa} = \begin{pmatrix} \dot{\varepsilon} & 0 & 0 \\ 0 & -\dot{\varepsilon} & 0 \\ 0 & 0 & 0 \end{pmatrix} \tag{3}$$

where $\dot{\varepsilon}$ is the dimensionless strain rate rescaled The stress tensor (rescaled by $ck_BT$) is calculated for a multi-chain system as [6]

$$\boldsymbol{\sigma} = \frac{1}{N_c}\left[\sum_{N_c}\sum_{\nu=1}^{N_b-1}\langle \mathbf{Q}_\nu \, \mathbf{F}^c_\nu \rangle\right], \tag{4}$$

where $\mathbf{Q}_\nu$ is the $\nu$-th connector vector and $\mathbf{F}^c_\nu$ is the corresponding FENE connector force. The angle brackets represent an ensemble average. The dimensionless polymer contribution to the extensional viscosity of polymer solutions is

$$\overline{\eta}_{\mathrm{p}} = -\frac{\sigma_{xx} - \sigma_{yy}}{\dot{\epsilon}}\,. \tag{5}$$

Simulations were performed for two different initial ensembles of the polymer molecules, namely, an initially coiled state where chain configurations are sampled from an equilibrium dstribution, and an initially stretched state where all polymer chains are initially stretched to 90% of their contour length. Simulations were run for either ensemble at each imposed extensional strain-rate until the normal stress difference reached a plateau that is steady for several Hencky strain units. The ensemble average was obtained over 100 independent trajectories. Simulations were run with $N_b = 20$, $N_{\mathrm{K}} = 1300$ and $h^* = 0.25$. The $c/c^*$, $N_c$ and $L$ (rescaled by equilibrium root-mean-squared spring length) values are shown in Table II. The $c^*$ values are based on the equilibrium radius of gyration which in the absence of excluded volume interactions is calculated as

$$R_g^2 = \frac{b}{b+5}\,\frac{N_b^2-1}{2N_b}\,,$$

where $b = 3\,(N_{\mathrm{K}}/N_s) - 5$ is the FENE parameter representing the dimensionless polymer contour length underlying each spring. The relaxation time $\lambda_0$ was estimated from the critical strain-rate $\dot{\varepsilon}_{\mathrm{CS}}$ for the coil–stretch transition as $\lambda_0 = 1/(2\,\dot{\varepsilon}_{\mathrm{CS}})$. The $\dot{\varepsilon}_{\mathrm{CS}}$ at each $c/c^*$ was estimated as the midpoint between the strain-rates before and after the transition.

TABLE II. Dimensionless parameters in multi-chain Brownian Dynamics simulations

| $c/c^*$ | $N_c$ | $L$ |
|---|---|---|
| $1.1 \times 10^{-10}$ | 3 | 15225 |
| 0.05 | 33 | 43.92 |
| 0.1 | 50 | 40.27 |
| 0.5 | 58 | 24.69 |
| 1.3 | 85 | 20.46 |
| 2.0 | 111 | 19.38 |

## AVERAGE FRICTION COEFFICIENT FROM BLOB THEORY

This section summarizes the key scaling results and algorithm for the average friction coefficient $\zeta$ presented by Prabhakar et al. [7]. The ratio of $\zeta$ to $\zeta_{\mathrm{Z}}$ is obtained as a function of the normalized stretch $R/R_0$ and concentration $c/c^*$. The other dimensionless parameters required for the calculation are $N_{\mathrm{K}}$ and $h^*_{\mathrm{K}}$. Calculation of $\zeta_{\mathrm{Z}}$ additionally needs $\eta_{\mathrm{s}}$ and $b_{\mathrm{K}}$. Excluded volume interactions are neglected for the sake of simplicity, and the equations presented below are therefore only strictly valid for theta solutions. Entanglements and reptation are also neglected. Given $R/R_0$ and $c/c^*$, we first determine whether the tension blob (t-blob) or the correlation blob (c-blob) is smaller *i.e.* which of these is the core blob. This depends on the location of the system on the stretch-concentration state space shown in Fig. 1. The horizontal axis in that figure represents the equilibrium state of polymer solutions consisting of isotropic coils while the vertical axis represents partially stretched chains at infinite dilution. The maximum stretch ratio $R/R_0$ possible is $L/R_0 = \sqrt{N_{\mathrm{K}}}$. In a fully stretched chain, the t-blob has the same size of a single Kuhn segment. When a c-blob has the same size as a Kuhn segment, all intramolecular HI is completely screened irrespective of chain conformation. This can be shown to occur when $c/c^* = \sqrt{N_{\mathrm{K}}}$. Polymer solutions above this concentration are in the concentrated-solution regime, where $\zeta = \zeta_{\mathrm{R}}$. The state space in Fig. 1 is thus defined by the ranges $1 \leq R/R_0 \leq \sqrt{N_{\mathrm{K}}}$ and $0 \leq c/c^* \leq \sqrt{N_{\mathrm{K}}}$.

There are three principal regions in this state space. The dilute regime is defined by the regime where $c/c^* < (R/R_0)^{-3}$ where only t-blobs are present. In the intermediate semidilute regime where $(R/R_0)^{-3} < c/c^* < R/R_0$, t-blobs are the core blobs and hydrodynamic screening is weak. C-blobs are the core blobs in the semidilute regime with strong hydrodynamic

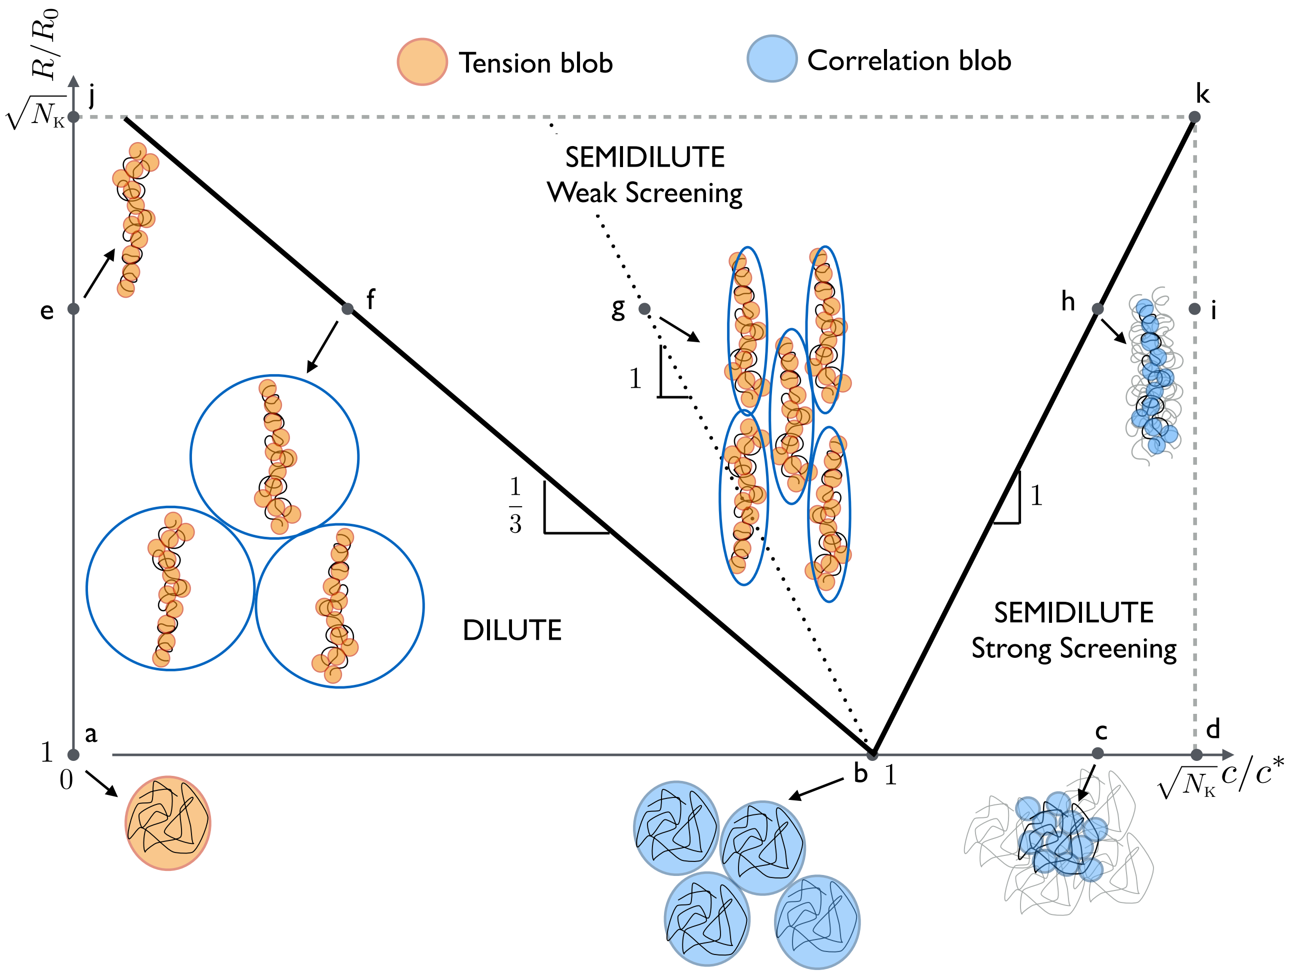


FIG. 1. Stretch–concentration state space for polymer solutions showing the dilute regime, and the semidilute regimes with weak and strong hydrodynamic screening. (a) Isolated, equilibrium coils described by Zimm hydrodynamics: each coil is a single t-blob. (b) Equilibrium coils at critical overlap: each coil is a single c-blob. (c) Semidilute coils with c-blobs smaller than coil size. (d) Concentrated solution with c-blobs of the same size as a Kuhn segment (e) Isolated, stretched chains with t-blobs. (f) Chains of t-blobs begin to interact hydrodynamically with a screening length approximately equal to chain length. (g) Chains of t-blobs at critical transverse overlap with anisotropic c-blobs larger than t-blobs. (h) Transition of stretched chains from weak- to strong hydrodynamic screening with c-blobs as small as t-blobs. (i) Concentrated solution of stretched chains with c-blobs of the same size as a Kuhn segment. (j) Fully stretched chains with t-blobs as small as a single Kuhn segment. (k) Concentrated solution of fully stretched chains.

screening; this occurs when $c/c^* > R/R_0$. The number and size of the core blobs are given by:

$$\begin{cases} N_{\rm t} = (R/R_0)^2\,; \quad \xi_{\rm t}/R_0 = (R/R_0)^{-1}\,, & \text{if } c/c^* \leq (R/R_0)\,; \\ N_{\rm c} = (c/c^*)^2\,; \quad \xi_{\rm c}/R_0 = (c/c^*)^{-1}\,, & \text{if } c/c^* \geq R/R_0\,. \end{cases} \tag{6}$$

Scaling relationships for the friction coefficient deep inside each of the regimes in state space are the following:

$$\zeta = \begin{cases} \zeta_{\rm Z}\,, & \text{if } c/c^* \ll 1 \text{ and } R/R_0 = 1 \text{ (dilute and coiled)}\;; \\ \dfrac{\zeta_{\rm t}\,N_{\rm t}}{\ln{(2\,N_{\rm t})}}\,, & \text{if } c/c^* \ll (R/R_0)^{-3} \text{ (dilute and stretched)}\;; \\ \dfrac{\zeta_{\rm t}\,N_{\rm t}}{\ln{(2\,\chi/\xi_{\rm t})}}\,, & \text{if } (R/R_0)^{-3} \ll c/c^* \ll R/R_0 \text{ (weakly screened)}\,; \\ \zeta_{\rm c}\,N_{\rm c}\,, & \text{if } R/R_0 \ll c/c^* \ll \sqrt{N_{\rm K}} \text{ (strongly screened)}\,; \\ \zeta_{\rm R}\,, & \text{if } c/c^* \geq \sqrt{N_{\rm K}} \text{ (concentrated)}\,; \end{cases} \tag{7}$$

In the equations above, $\chi$ is the hydrodynamic screening in the weak-screening regime and the ratio,

$$\frac{\chi}{\xi_{\rm t}} = \left[\frac{1}{\phi_{\rm t}}\ln\left(\frac{1}{\phi_{\rm t}}\right)\right]^{1/2}\,, \tag{8}$$

where the volume fraction of t-blob poles is

$$\phi_{\rm t} \,=\, c\,R\,\xi_{\rm t}^2 \,=\, \frac{c/c^*}{R/R_0}\,. \tag{9}$$

Neither chain stretching nor intermolecular screening are felt inside any core blob within which the chain structure is an ideal random walk and intramolecular HI is dominant. If the number of segments within a core blob is $N \leq N_{\rm K}$, its size $\xi = b_{\rm K}N^{1/2}$ is taken as an estimate of its diameter. Intramolecular HI leads to partial draining, and the draining ratio

$$\alpha = \frac{\zeta_{\rm blob}}{\eta_{\rm s}\,\xi}\,, \tag{10}$$

measures partial draining. The friction coefficient of a non-draining blob would be the same as that of a rigid sphere of the same size *i.e.* $\alpha = 3\pi$. In general, $\alpha$ is a function of $N$ and

$h_{\rm K}^*$. In the limit of infinitely large $N$, $\alpha$ approaches a value smaller than $3\pi$. At equilibrium and infinite dilution, the whole coil is a single blob. The Zimm friction coefficient therefore is $\zeta_{\rm Z} = \alpha(h_{\rm K}^*, N_{\rm K})\, \eta_{\rm s} R_0$. As a core blob shrinks in size towards a single Kuhn segment, $\zeta_{\rm blob}$ approaches the friction coefficient of a single Kuhn segment $6\pi^{3/2}\eta_{\rm s} h_{\rm K}^* b_{\rm K}$ and $\alpha$ approaches $6\pi^{3/2} h_{\rm K}^*$. The draining function $\alpha(h_{\rm K}^*, N)$ has been estimated by Prabhakar et al. [7] using the Kirkwood-Riseman approximation (Fig. 2). Using this function, the value of $\zeta_{\rm t}$ or $\zeta_{\rm c}$ in Eqn. (7) can be calculated with $N = N_{\rm K}/N_{\rm t}$ or $N_{\rm K}/N_{\rm c}$, respectively, for any given $h_{\rm K}^*$.

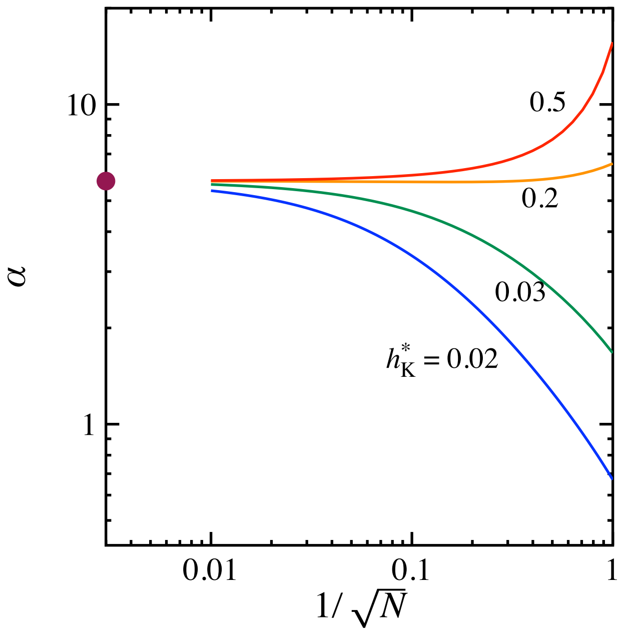


FIG. 2. The draining function for several values of $h_{\rm K}^*$; the circle represents the value $\alpha_\infty \approx 5.8$ in the limit of infinite chains.

We set the friction coefficient of equilibrium coils to be

$$\zeta_0 = \begin{cases} \zeta_{\rm Z}\,, & \text{if } c/c^* \leq 1\,, \\ \zeta_{\rm c}\, N_{\rm c}\,, & \text{if } 1 < c/c^* \leq \sqrt{N_{\rm K}}\,, \\ \zeta_{\rm R}\,, & \text{if } c/c^* \geq \sqrt{N_{\rm K}} \end{cases} \tag{11}$$

Everywhere in the strong screening regime, we set $\zeta = \zeta_{\rm c} N_{\rm c}$ with $\xi_{\rm c}$ and $N_{\rm c}$ calculated using Eqn. (6) above, and with $\zeta_{\rm c} = \alpha(h_{\rm K}^*, N_{\rm K}/N_{\rm c})\, \eta_{\rm s}\, \xi_{\rm c}$. For partially stretched chains in the dilute and weak-screening regimes where t-blobs are the core blobs$\xi_{\rm t}$ and $N_{\rm t}$ are calculated using Eqn. (6), and $\zeta_{\rm t} = \alpha(h_{\rm K}^*, N_{\rm K}/N_{\rm t})\, \eta_{\rm s}\, \xi_{\rm t}$. We use the following equations to interpolate

between the scaling results and achieve $\zeta = \zeta_c N_c$ on the boundary between the weak- and strong-screening regimes:

$$\zeta = \frac{\zeta_t N_t}{G_1/G_2} \;, \tag{12}$$

where,

$$G_1 = 1 + \ln\left[\frac{A + (B-1)\,J}{A + B}\right], \tag{13}$$

$$G_2 = 1 + \ln\left[\frac{B}{(1/A) + B}\right], \tag{14}$$

$$\tag{15}$$

and $A = R/\xi_t$ is the aspect ratio of the t-blob pole, $B = 1 + \chi/\xi_t$ and $C = A - 1$. The function

$$J = 1 + \left[\frac{(1/2)\,C + (2/e)\,C^2}{C + 1}\right], \tag{16}$$

is a rational function in the aspect ratio $A$, such that $J = 1$ when $A = 1$ (at equilibrium) and $J \to (2/e)\,A$ when $A \to \infty$. On weak/strong-screening boudnary, $\chi/\xi_t = 0$, and $B = 1$. Further, if $A \gg 1$, then $G_1/G_2 \approx 1$, recovering the required value at that boundary. As $c/c^* \to 0$, $\chi$ and $B \to \infty$. Hence, in the dilute limit at $c/c^* \to 0$, $G_1 \to 1 + \ln J$ and $G_2 \to 1$. The interpolation scheme produces shallow unphysical local minima when $R/R_0$ is close to 1 or near the weak/strong screening boundary. To remove these, we calculate first $\zeta$ with the interpolation formula above, and then choose $\max(\zeta, \zeta_0)$ as the final value of the friction coefficient. Figure 3 show typical plots of the ratio $\zeta/\zeta_Z$ as a function of $R/R_0$ and $c/c^*$.

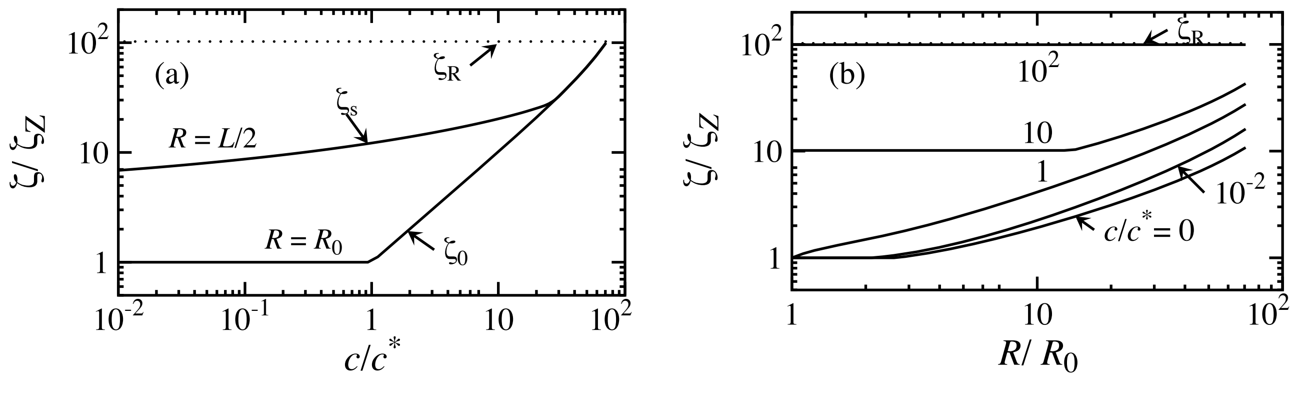


FIG. 3. Friction coefficient as a function of (a) concentration and (b) end-to-end polymer stretch for $N_K = 5 \times 10^3$ and $h_K^* = 0.25$. The dotted line represents the Rouse value $\zeta_R$.

[1] R. Prabhakar, J. R. Prakash, and T. Sridhar. A successive fine-graining scheme for predicting the rheological properties of dilute polymer solutions. *J. Rheol.*, 48:1251–1278, 2004.

[2] R. K. Gupta, D. A. Nguyen, and T. Sridhar. Extensional viscosity of dilute polystyrene solutions: Effect of concentration and molecular weight. *Phys. Fluids*, 12:1296–1318, 2000.

[3] W. W. Graessley. Polymer chain dimensions and the dependence of viscoelastic properties on concentration, molecular weight and solvent power. *Polymer*, 21:258–262, 1980.

[4] A. Jain, P. Sunthar, B. Dnweg, and J. R. Prakash. Optimization of a Brownian-dynamics algorithm for semidilute polymer solutions. *Phys. Rev. E*, 85:066703, 2012.

[5] A. Jain, C. Sasmal, R. Hartkamp, B. D. Todd, and J. R. Prakash. Brownian dynamics simulations of planar mixed flows of polymer solutions at finite concentrations. *Chem. Eng. Sci.*, 121:245– 257, 2015.

[6] C. Stoltz, J. J. de Pablo, and M. D. Graham. Concentration dependence of shear and extensional rheology of polymer solutions: Brownian dynamics simulations. *J. Rheol.*, 50:137–167, 2006.

[7] R. Prabhakar, S. Gadkari, T. Gopesh, and M. J. Shaw. Influence of stretching induced self-concentration and self-dilution on coil-stretch hysteresis and capillary thinning of unentangled polymer solutions. *J. Rheol.*, page in press, 2016.
